# Supplementary material for: Evaluating Language Models on Cross-Language Code Functional Equivalence
Source: arXiv:2608.23961 source file (2026-08-25)
Supplement: Supplementary file 1 [file Appendix.tex]

\section{Supplementary Analysis Materials}
